# Supplementary material for: Set-Based Tests for Genetic Association Using the Generalized Berk-Jones Statistic
Source: arXiv:1710.02469 ancillary file (2017-10-11)
Supplement: Supplementary file 1 [file supp_materials.pdf]

# Supplementary Materials for "Set-Based Tests for Genetic Association Using the Generalized Berk-Jones Statistic"

Ryan Sun and Xihong Lin

September 20, 2017

**Supplement A:** Proof of Theorem 1 from Section 3.3.

**Supplement B:** Exact p-value calculation using equation (5) from Section 3.4.

**Supplement C:** Complete simulation parameters from Section 5.

## Supplement A: Proof of Theorem 1 from Section 3.3

We are interested in the variance of

$$\begin{aligned} S(t) &= \sum_{k=1}^{d} \mathbf{1}\left(|Z_k| \geq t\right), \\ \mathbf{Z} &\sim MVN\left(\mu \cdot \mathbf{J}_d, \mathbf{\Sigma}\right), \end{aligned}$$

where the diagonal elements of $\mathbf{\Sigma}$ are all 1. The variance can be decomposed as

$$\begin{aligned} \mathrm{Var}\left\{S(t)\right\} &= d\lambda(1-\lambda) + 2\sum_{1\leq k<l\leq d}\left\{\Pr\left(|Z_k|, |Z_l| \geq t\right) - \lambda^2\right\}, \\ \lambda &= 1 - \left\{\Phi\left(t-\mu\right) - \Phi(-t-\mu)\right\}. \end{aligned}$$

The summation can be written as

$$\begin{aligned} 2\sum_{1\leq k<l\leq d}\left\{\Pr\left(|Z_k|, |Z_l| \geq t\right) - \lambda^2\right\} &= 2\sum_{1\leq k<l\leq d}\Pr\left(Z_k, Z_l \geq t\right) \\ &\quad +2\sum_{1\leq k<l\leq d}\Pr\left(Z_k, Z_l \leq -t\right) \\ &\quad +2\sum_{1\leq k<l\leq d}\Pr\left(Z_k \geq t, Z_l \leq -t\right) \\ &\quad +2\sum_{1\leq k<l\leq d}\Pr\left(Z_k \leq -t, Z_l \geq t\right) \\ &\quad -d(d-1)\lambda^2. \end{aligned}$$

Each of the four probabilities above can be reexpressed using the standard Mehler kernel for the bivariate normal distribution. For example, the first probability is:

$$\begin{aligned} & 2\sum_{1\leq k<l\leq d}\Pr\left(Z_k, Z_l \geq t\right) \\ = \;& 2\sum_{1\leq k<l\leq d}\int_t^\infty\int_t^\infty \frac{1}{2\pi\sqrt{1-\rho_{k,l}^2}}\exp\left[-\frac{1}{2(1-\rho_{k,l}^2)}\left\{(z_k-\mu)^2 - 2\rho_{k,l}(z_k-\mu)(z_l-\mu) + (z_l-\mu)^2\right\}\right]dz_k dz_l, \\ = \;& 2\sum_{1\leq k<l\leq d}\int_t^\infty\int_t^\infty \phi(z_k-\mu)\phi(z_l-\mu)\sum_{r=0}^{\infty}\frac{\rho_{k,l}^r}{r!}H_r(z_k-\mu)H_r(z_l-\mu)dz_k dz_l, \\ = \;& 2\sum_{1\leq k<l\leq d}\left\{\bar{\Phi}(t-\mu)^2 + \int_t^\infty\int_t^\infty \phi(z_k-\mu)\phi(z_l-\mu)\sum_{r=1}^{\infty}\frac{\rho_{k,l}^r}{r!}H_r(z_k-\mu)H_r(z_l-\mu)dz_k dz_l\right\}, \\ = \;& 2\sum_{1\leq k<l\leq d}\left\{\bar{\Phi}(t-\mu)^2 + \phi(t-\mu)^2\sum_{r=1}^{\infty}\frac{\rho_{k,l}^r}{r!}H_{r-1}(t-\mu)^2\right\}, \end{aligned}$$

$$
\begin{aligned}
&= d(d-1)\bar{\Phi}(t-\mu)^2 + 2\phi(t-\mu)^2 \sum_{r=1}^{\infty} \frac{1}{r!} H_{r-1}(t-\mu)^2 \left( \sum_{1\le k<l\le d} \rho_{k,l}^r \right), \\
&= d(d-1)\bar{\Phi}(t-\mu)^2 + 2\phi(t-\mu)^2 \sum_{r=1}^{\infty} \frac{1}{r!} H_{r-1}(t-\mu)^2 \left( \frac{d(d-1)}{2} \bar{\rho^r} \right), \\
&= d(d-1) \left\{ \bar{\Phi}(t-\mu)^2 + \phi(t-\mu)^2 \sum_{r=1}^{\infty} \frac{\bar{\rho^r}}{r!} H_{r-1}(t-\mu)^2 \right\}, \\
\bar{\rho^r} &= \frac{2}{d(d-1)} \sum_{1\le k<l\le d} \rho_{k,l}^r.
\end{aligned}
$$

Here $\phi(x)$ represents the density function of $N(0,1)$ distribution and $\rho_{k,l}$ is the $(k,l)$ element of $\mathbf{\Sigma}$. We skip the similar derivation for the other three probabilities and give only the final expressions:

$$
\begin{aligned}
2\sum_{1\le k<l\le d} \Pr\left(Z_k, Z_l \le -t\right) &= d(d-1) \left\{ \Phi(-t-\mu)^2 + \phi(-t-\mu)^2 \sum_{r=1}^{\infty} \frac{\bar{\rho^r}}{r!} H_{r-1}(-t-\mu)^2 \right\}, \\
2\sum_{1\le k<l\le d} \Pr\left(Z_k \le -t, Z_l \ge t\right) &= d(d-1) \left\{ \Phi(-t-\mu)\bar{\Phi}(t-\mu) \right\} \\
&\quad -d(d-1) \left\{ \phi(-t-\mu)\phi(t-\mu) \sum_{r=1}^{\infty} \frac{\bar{\rho^r}}{r!} H_{r-1}(-t-\mu) H_{r-1}(t-\mu) \right\}, \\
&= 2\sum_{1\le k<l\le d} \Pr\left(Z_k \ge t, Z_l \le -t\right).
\end{aligned}
$$

So in total we have

$$
\begin{aligned}
2\sum_{1\le k<l\le d} \left\{ \Pr\left(|Z_k|, |Z_l| \ge t\right) - \lambda^2 \right\} &= d(d-1) \left\{ \bar{\Phi}(t-\mu)^2 + \phi(t-\mu)^2 \sum_{r=1}^{\infty} \frac{\bar{\rho^r}}{r!} H_{r-1}(t-\mu)^2 \right\} \\
&\quad +d(d-1) \left\{ \Phi(-t-\mu)^2 + \phi(-t-\mu)^2 \sum_{r=1}^{\infty} \frac{\bar{\rho^r}}{r!} H_{r-1}(-t-\mu)^2 \right\} \\
&\quad +2d(d-1) \left\{ \Phi(-t-\mu)\bar{\Phi}(t-\mu) \right\} \\
&\quad -2d(d-1) \left\{ \phi(-t-\mu)\phi(t-\mu) \sum_{r=1}^{\infty} \frac{\bar{\rho^r}}{r!} H_{r-1}(-t-\mu) H_{r-1}(t-\mu) \right\} \\
&\quad -d(d-1) \left\{ \bar{\Phi}\left(t-\mu\right) + \Phi(-t-\mu) \right\}^2, \\
&= d(d-1) \left\{ \phi(t-\mu)^2 \sum_{r=1}^{\infty} \frac{\bar{\rho^r}}{r!} H_{r-1}(t-\mu)^2 \right\} \\
&\quad +d(d-1) \left\{ \phi(-t-\mu)^2 \sum_{r=1}^{\infty} \frac{\bar{\rho^r}}{r!} H_{r-1}(-t-\mu)^2 \right\} \\
&\quad -2d(d-1) \left\{ \phi(-t-\mu)\phi(t-\mu) \sum_{r=1}^{\infty} \frac{\bar{\rho^r}}{r!} H_{r-1}(-t-\mu) H_{r-1}(t-\mu) \right\}.
\end{aligned}
$$

Put it all back together for the result given in the theorem.

# Supplement B: Exact p-value calculation using equation (5) from Section 3.4.

We are interested in calculating the probability

$$\Pr(G_d \geq g) \;=\; 1 - \Pr\left\{\forall j = 1, 2, ..., d : |Z|_{(j)} \leq b_j \middle| \mathbf{Z} \sim MVN(\mathbf{0}, \mathbf{\Sigma})\right\}.$$

Using the law of total probability, our quantity of interest is

$$\begin{aligned}&\Pr\left\{\forall j = 1, 2, ..., d : |Z|_{(j)} \leq b_j \middle| \mathbf{Z} \sim MVN(\mathbf{0}, \mathbf{\Sigma})\right\}\\ =\;& \sum_{\mathbf{a}\in\mathcal{A}} \Pr\left\{\forall j = 1, 2, ..., d : |Z|_{(j)} \leq b_j, |Z|_{(j)} = |Z_{a_j}| \middle| \mathbf{Z} \sim MVN(\mathbf{0}, \mathbf{\Sigma})\right\},\end{aligned}$$

where $\mathbf{a} = (a_1, a_2, ..., a_d)$ and $\mathcal{A}$ is the set of all $d!$ possible permutations of the integers from 1 to $d$. Thus the p-value can be expressed as

$$\begin{aligned}&\Pr(G_d \geq g)\\ =\;& 1 - \sum_{\mathbf{a}\in\mathcal{A}} \Pr\left\{0 \leq |Z_{a_1}| \leq b_1, |Z_{a_1}| \leq |Z_{a_2}| \leq b_2, ...., |Z_{a_{d-1}}| \leq |Z_{a_d}| \leq b_d \middle| \mathbf{Z} \sim MVN(\mathbf{0}, \mathbf{\Sigma})\right\}.\end{aligned}$$

At this point it is apparent that we will need some sort of distribution function for $\mathbf{Y} = (Y_1, Y_2, ..., Y_d) = (|Z_1|, |Z_2|, ..., |Z_d|)$, where $\mathbf{Y}$ is the result of applying the absolute value operator on every element of $\mathbf{Z}$. $\mathbf{Y}$ is also known as the multivariate half-normal distribution. If $\mathbf{Z} \sim MVN(\mathbf{0}, \mathbf{\Sigma})$, then the probability density function of $\mathbf{Y}$ can be written as

$$\begin{aligned} f_{\mathbf{Y}}(\mathbf{y}) &= \sum_{\mathbf{s}\in S} (2\pi)^{-\frac{d}{2}} |\mathbf{\Sigma}_s|^{-\frac{1}{2}} \exp\left\{-\frac{1}{2}\mathbf{y}^T \mathbf{\Sigma}_s^{-1} \mathbf{y}\right\}, \qquad \text{(S.1)}\\ S &= \{(\delta_1, ..., \delta_d) : \delta_j = \pm 1 \forall j = 1, 2, ..., d\},\\ \mathbf{\Lambda_s} &= \{\text{diag}(\mathbf{s})\},\\ \mathbf{\Sigma_s} &= \mathbf{\Lambda_s \Sigma \Lambda_s}.\end{aligned}$$

Note that there are $2^d$ elements in $S$. With the use of (S.1), the p-value can be expressed as a $d$-dimensional integral:

$$\Pr(G \geq g) = 1 - \sum_{\mathbf{a}\in\mathcal{A}} \sum_{\mathbf{s}\in S} \int_0^{b_1} \int_{Y_1}^{b_2} ... \int_{Y_{d-1}}^{b_d} (2\pi)^{-\frac{d}{2}} |\mathbf{\Sigma}_{\mathbf{s}}^{(\mathbf{a})}|^{-\frac{1}{2}} \exp\left\{-\frac{1}{2}\mathbf{y}^T \left(\mathbf{\Sigma}_{\mathbf{s}}^{(\mathbf{a})}\right)^{-1} \mathbf{y}\right\} dY_d ... dY_1. \qquad \text{(S.2)}$$

By the use of $\mathbf{\Sigma}_{\mathbf{s}}^{(\mathbf{a})}$ we mean the variance matrix that is permuted to account for the ordering $\mathbf{a}$. It can be defined as:

$$\begin{aligned}
\mathbf{\Sigma}_{\mathbf{s}}^{(\mathbf{a})} &= \mathbf{\Lambda_s P^{(a)} \Sigma P^{(a)\mathit{T}} \Lambda_s}, \\
\mathbf{P}^{(\mathbf{a})} &= \begin{pmatrix} \mathbf{e}_{a_1}^T \\ \mathbf{e}_{a_2}^T \\ . \\ . \\ \mathbf{e}_{a_d}^T \end{pmatrix},
\end{aligned}$$

where $\mathbf{e}_j$ denotes the $d \times 1$ vector with a 1 in the $j$th position and 0 everywhere else. Although equation (S.2) appears to be calculable through many calls to a multivariate normal distribution solver, the lower bounds are functions of variables in the integration, which is not a feature supported by many statistical computing packages. To put the expression into a form more accessible for computation, we can reinterpret the $d$-dimensional integral:

$$\begin{aligned}
&\int_0^{b_1}\int_{Y_1}^{b_2} ... \int_{Y_{d-1}}^{b_d} (2\pi)^{-\frac{d}{2}} |\mathbf{\Sigma}_{\mathbf{s}}^{(\mathbf{a})}|^{-\frac{1}{2}} \exp\left\{-\frac{1}{2}\mathbf{y}^T \left(\mathbf{\Sigma}_{\mathbf{s}}^{(\mathbf{a})}\right)^{-1} \mathbf{y}\right\} dY_d...dY_1 \\
= \ & \Pr\left\{0 \le Y_1 \le b_1, Y_1 \le Y_2 \le b_2, ..., Y_{d-1} \le Y_d \le b_d \middle| \mathbf{Y} \sim MVN\left(\mathbf{0}, \mathbf{\Sigma}_{\mathbf{s}}^{(\mathbf{a})}\right)\right\}, \\
= \ & \Pr\left\{0 \le Y_1 \le b_1, Y_2 \le b_2, ..., Y_d \le b_d, Y_2 - Y_1 \ge 0, ..., Y_d - Y_{d-1} \ge 0 \middle| \mathbf{Y} \sim MVN\left(\mathbf{0}, \mathbf{\Sigma}_{\mathbf{s}}^{(\mathbf{a})}\right)\right\}. \quad \text{(S.3)}
\end{aligned}$$

To be clear, equation (S.3) is meant to show how the integral of equation (S.2) can be viewed as a simpler probability if we reinterpret $\mathbf{Y}$ as possessing a multivariate normal distribution instead of its true multivariate half-normal distribution. Equation (S.3) is simpler because the bounds are all constants, which is a form more amenable to most statistical software. Our final step to simplify the quantity for computation is to introduce the vector $\mathbf{T} = (T_1, T_2, ..., T_{2d-1})$ so that

$$\begin{aligned}
&\Pr\left\{0 \le Y_1 \le b_1, Y_2 \le b_2, ..., Y_d \le b_d, Y_2 - Y_1 \ge 0, ..., Y_d - Y_{d-1} \ge 0 \middle| \mathbf{Y} \sim MVN(\mathbf{0}, \mathbf{\Sigma}_s^{(a)})\right\} \\
= \ & \Pr\left\{0 \le T_1 \le b_1, T_2 \le b_2, ..., T_d \le b_d, T_{d+1} \ge 0, ..., T_{2d-1} \ge 0 \middle| \mathbf{T} \sim MVN\left(\mathbf{0}_{(2d-1)\times 1}, \mathbf{\Delta}_d \mathbf{\Sigma}_{\mathbf{s}}^{(\mathbf{a})} \mathbf{\Delta}_d^T\right)\right\}, \\
\mathbf{\Delta}_d \ = \ & \begin{pmatrix} \mathbf{I}_{d\times d} \\ \mathbf{D} \end{pmatrix}_{(2d-1)\times d},
\end{aligned}$$

$$
\mathbf{D} = \begin{pmatrix} -1 & 1 & & & & \\ & -1 & 1 & & & \\ & & \cdot & \cdot & & \\ & & \cdot & \cdot & & \\ & & & & -1 & 1 \end{pmatrix}_{(d-1)\times d} .
$$

The final p-value is given by

$$
\begin{aligned}
\Pr\left(G_d \geq g\right) &= 1 - \sum_{\mathbf{a}\in\mathcal{A}} \sum_{\mathbf{s}\in S} \Pr\left(\mathbf{L} \leq \mathbf{T}_{\mathbf{a},\mathbf{s}} \leq \mathbf{U}\right), \qquad \text{(S.4)} \\
\mathbf{T}_{\mathbf{a},\mathbf{s}} &\sim MVN\left(\mathbf{0}_{(2d-1)\times 1}, \mathbf{\Delta}_d \mathbf{\Sigma}_{\mathbf{s}}^{(\mathbf{a})} \mathbf{\Delta}_d^T\right), \\
\mathbf{L} &= (0, \underbrace{-\infty, ..., -\infty}_{d-1}, \underbrace{0, ..., 0}_{d-1}), \\
\mathbf{U} &= (b_1, b_2, ..., b_d, \underbrace{\infty, ..., \infty}_{d-1}).
\end{aligned}
$$

Equation (S.4) gives us the integral bounds as constants, at a cost of increasing the dimension of the multivariate normal distribution of interest from $d$ to $2d-1$. This final expression can be used in any number of computing packages to produce the desired probability.

# Supplement C: Complete simulation parameters from Section 5.

Below we give the effect sizes of the causal SNPs for the simulations using SNPs with predetermined correlation structures.

Supplementary Table 1: Effect sizes $\beta_j$ for each set of simulations in Figures 2 and 3. For a given number of causal SNPs, all causal SNPs have the same effect size.

| **Correlation** | | | **Number of Causal SNPs** | | | | | | | | | |
|---|---|---|---|---|---|---|---|---|---|---|---|---|
| $\rho_1$ | $\rho_2$ | $\rho_3$ | 1 | 2 | 3 | 4 | 5 | 6 | 7 | 8 | 9 | 10 |
| 0.0 | 0.0 | 0.0 | 0.120 | 0.100 | 0.090 | 0.090 | 0.090 | 0.090 | 0.090 | 0.090 | 0.090 | 0.090 |
| 0.3 | 0.0 | 0.0 | 0.110 | 0.080 | 0.060 | 0.050 | 0.040 | 0.040 | 0.035 | 0.030 | 0.030 | 0.030 |
| 0.3 | 0.0 | 0.3 | 0.110 | 0.090 | 0.060 | 0.050 | 0.050 | 0.040 | 0.030 | 0.030 | 0.030 | 0.030 |
| 0.3 | 0.3 | 0.3 | 0.100 | 0.070 | 0.050 | 0.040 | 0.035 | 0.030 | 0.025 | 0.025 | 0.025 | 0.025 |

And finally we give the effect sizes of the causal SNPs for simulations using HAPGEN2-generated blocks of 40 SNPs on chromosome 5.

Supplementary Table 2: Effect sizes $\beta_j$ for simulation with HAPGEN2-generated blocks of 40 SNPs on chromosome 5 (Figure 4). For a given number of causal SNPs, all causal SNPs have the same effect size.

| **Number of Causal SNPs** | | | | | | | |
|---|---|---|---|---|---|---|---|
| 1 | 2 | 3 | 4 | 5 | 6 | 7 | 8 |
| 0.16 | 0.14 | 0.12 | 0.12 | 0.11 | 0.11 | 0.10 | 0.10 |
